# Supplementary material for: Attraction-enhanced emergence of friction in colloidal matter
Source: arXiv:2209.12703 ancillary file (2025-08-11)
Supplement: Supplementary file 1 [file SI.pdf]

# Supplemental Material

Berend van der Meer[1,2], Taiki Yanagishima[2,3], Roel P. A. Dullens[1,2]
[1] *Institute for Molecules and Materials, Radboud University, Heyendaalseweg 135, 6525 AJ, Nijmegen, The Netherlands*
[2] *Department of Chemistry, Physical and Theoretical Chemistry Laboratory, University of Oxford, South Parks Road, Oxford OX1 3QZ, United Kingdom and*
[3] *Department of Physics, Graduate School of Science, Kyoto University, Kitashirakawa Oiwake-cho, Sakyo-ku, Kyoto, 606-8502, Japan*

## I. PARTICLE CHARACTERIZATION

*Scanning electron microscopy*

The size of the OCULI particles was determined using scanning electron microscopy (SEM). A drop of particle suspension was dried on a piece of silicon wafer at room temperature. The dried sample was subsequently sputter-coated with platinum in an argon atmosphere. The SEM images were recording using a JSM-6010LV SEM unit (JEOL, Japan) at an accelerating voltage of 20kV. These images were analysed using a standard circle finding algorithm that extracts positions and diameters of particles within the field-of-view. The particles have a diameter $\sigma_{\mathrm{SEM}}= 2.78$ $\mu$m with a polydispersity of 3.1%. Furthermore, the particles are spherical and appear smooth [Fig. S1(a)].

*Particle diameter during confocal microscopy*

In our confocal microscopy experiments we expect the OCULI particles to be slightly larger in diameter compared to the SEM-measurements due to swelling of particles in haloalkane solvents. Based on Ref. [1], in which the same particle system and a similar solvent mixture was used, we expect a $\sim$10% increase in particle diameter in our confocal microscopy experiments compared to the SEM value. To confirm this estimate for the particles size after swelling, we have i) analysed close-packed structures of particles in an attractive system, and ii) measured the translational and rotational diffusivity of a dilute suspension of particles.

In our colloid-polymer mixtures, we typically observe two-dimensional crystalline domains at the glass wall [Fig. S1(b)]. At higher polymer concentration we may expect these particles to be almost close-packed, allowing us to extract the particle diameter by determining the mean interparticle spacing. Using this approach we obtain a particle diameter of $\sigma = 3.02$ $\mu$m.

We corroborate this value by measuring the translational and rotational diffusivity of a dilute suspension of these particles ($\phi \approx 0.01$). In this experiment no depletant was added, resulting in a purely repulsive hard-sphere interaction between particles. The trajectories were recorded far away from surfaces to eliminate wall effects. The Brownian rotation of particles is characterized using the orientational auto-correlation function, which in the dilute limit decays exponentially:

$$C(t) = \langle \mathbf{u}_i(t) \cdot \mathbf{u}_i(0) \rangle = e^{-t/\tau_r}, \tag{S1}$$

where $\tau_r = 1/2D_r$ is the rotational relaxation time. Here,

$$D_r = \frac{k_B T}{\pi \eta \sigma^3} \tag{S2}$$

is the rotational diffusion constant with $\eta$ the effective solvent viscosity, $T$ the temperature, and $k_B$ the Boltzmann constant. The measured orientational auto-correlation function is shown in Fig. S1(c). Clearly, the measured orientational motion agrees perfectly with the expected exponential decay, yielding a rotational diffusion coefficient $D_r = 3.1 \times 10^{-2}\mathrm{s}^{-1}$.

Similarly, the translational Brownian motion is characterized by calculating the mean-squared displacement (MSD), which in the dilute limit increases linearly with time:

$$\langle \Delta r^2(t) \rangle = \langle [\mathbf{r}_i(t) - \mathbf{r}_i(0)]^2 \rangle = 6D_t t \tag{S3}$$

with

$$D_t = \frac{k_B T}{3\pi \eta \sigma} \tag{S4}$$

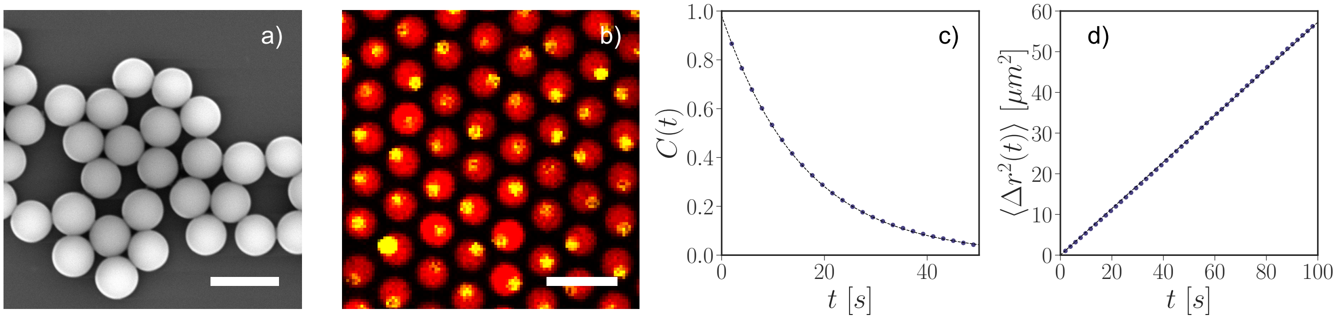


FIG. S1. (a) SEM picture of OCULI particles. Scale bar: 5 $\mu$m. (b) Two-channel confocal microscopy image of OCULI particles with attractive interactions forming an (almost) close-packed crystalline layer at the glass wall. Scale bar: 5 $\mu$m. (c) The orientational auto-correlation function and (d) the mean-square displacement for a dilute suspension of repulsive OCULI particles. Dashed lines are fits to Eqs. S1 & S3 from which the diffusion constants were extracted.

the translational diffusion constant. The MSD is shown in Fig. S1(d) and as expected increases linearly in time, yielding a translational diffusion coefficient $D_t = 9.5 \times 10^{-14}$ m$^2$/s.

Upon combining the extracted diffusion coefficients $D_t$ and $D_r$, we can simultaneously determine the particle diameter $\sigma = 3.04$ $\mu$m and effective solvent viscosity $\eta = 1.49$ mPa $\cdot$ s, simply by solving Eqs. S2 & S4. The particle diameters found in SEM and confocal microscopy are thus in excellent agreement upon correcting for a $\sim$10% change in size due to swelling in the solvent mixture.

## II. TRANSLATIONAL DYNAMICS OF PARTICLES IN COLLOIDAL GELS

To characterise our colloidal gels we monitor the translational dynamics of particles by measuring the MSD of the particles relative to their neighbours using

$$\langle \Delta r_{NR}^2(t) \rangle = \langle |\Delta \mathbf{r}_i(t) - \Delta \mathbf{r}_j(t)|^2 \rangle, \tag{S5}$$

where particles $i$ and $j$ are neighbors and $\Delta \mathbf{r}_i(t) = \mathbf{r}_i(t) - \mathbf{r}_i(0)$ denotes the displacement vector of particle $i$. Note that we use this two-particle MSD $\langle \Delta r_{NR}^2(t) \rangle$ as the single-particle MSD is dominated by correlated motion due to gel-network restructuring at larger length scales [2]. As shown in Fig. S2(a), the translational dynamics are characterised by slow dynamics characteristic for colloidal gels, where particle motion is largely arrested and a subdiffusive dynamics arises due to structural rearrangements underlying coarsening of the gel network. This "arrested" translational dynamics is also evident upon plotting a few typical trajectories at different attractive strengths [Fig. S2(b-d)]. Clearly, particles moves only a small amount compared to the interparticle spacing over the course of the experiment ( $\sim$1 hour).

## III. COORDINATION-DEPENDENT ORIENTATIONAL AUTOCORRELATION FUNCTION FOR THE SIMULATED ROUGH-PARTICLE SYSTEM

For the simulated rough-particle system, we calculate the coordination-dependent orientational autocorrelation function $C(Z, t)$ for a range of polymer reservoir densities $\rho_p \sigma^3$. Similarly to the experiments, we observe a clear slowing down of the orientational relaxation with increasing local coordination number [Fig. S3], which is especially pronounced at higher attractive strengths [Fig. S3(a-d)].

[1] T. Yanagishima, Y. Liu, H. Tanaka, and R. P. A. Dullens, Particle-level visualization of hydrodynamic and frictional couplings in dense suspensions of spherical colloids, Physical Review X **11**, 021056 (2021).
[2] J. M. van Doorn, J. Bronkhorst, R. Higler, T. van de Laar, and J. Sprakel, Linking particle dynamics to local connectivity in colloidal gels, Physical Review Letters **118**, 188001 (2017).

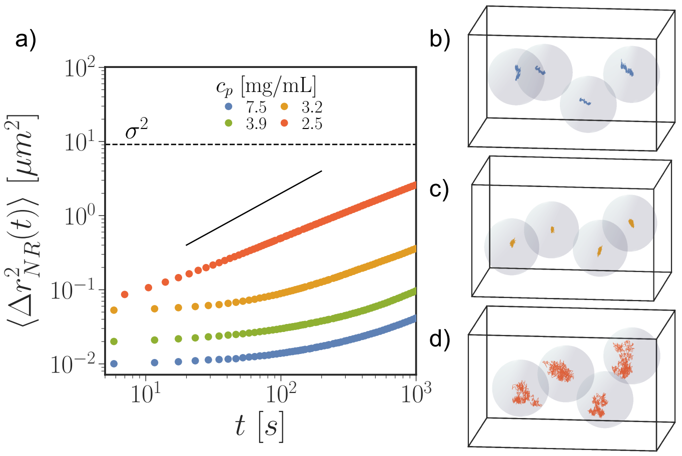


FIG. S2. Translational dynamics of particles in colloidal gels. (a) Neighbour-relative mean squared displacement of particle positions at different polymer concentrations. The translational motion of particles is arrested, giving rise to subdiffusive dynamics as indicated by the black line, which has a slope of 1. (b-d) This "arrested" translational motion is also illustrated by plotting the trajectories of a few neighboring particles for polymer concentrations of 7.5, 3.2 and 2.5 mg/mL (top to bottom). Particle outlines are drawn to scale.

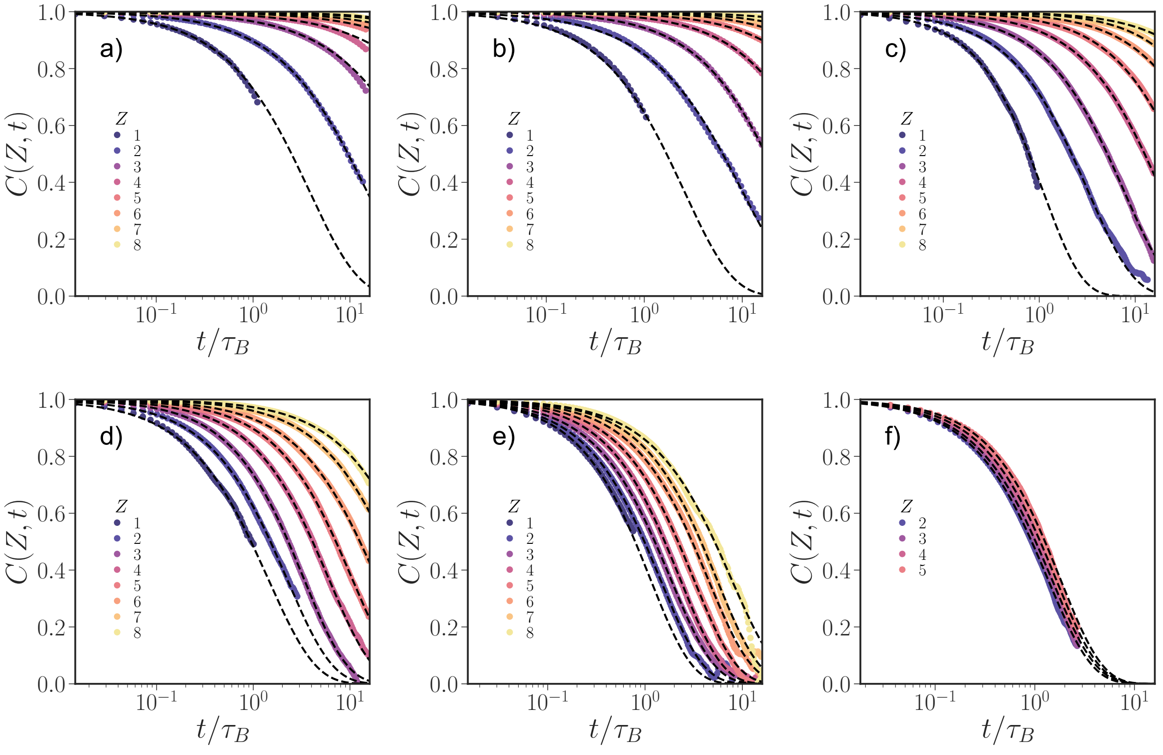


FIG. S3. The coordination-dependent orientational autocorrelation function $C(Z,t)$ for the simulated rough-particle system. In panels (a-f) the polymer reservoir density equals $\rho_p \sigma^3 = 4000$, 3500, 3000, 2500, 2000, and 1500, respectively. Dashed lines correspond to stretched-exponential fits.
